# Supplementary material for: How Contaminated Is Your Benchmark? Quantifying Dataset Leakage in Large Language Models with Kernel Divergence
Source: arXiv:2502.00678 source file (2025-05-20)
Supplement: Supplementary file 1 [file dataset_size.tex]

\section{Effect of Dataset Size}
\label{apdx:size}
